# Supplementary material for: Pros and Cons of the Bethe-Salpeter Formalism for Ground-State Energies
Source: arXiv:2002.04514 source file (2020-04-02)
Supplement: Supplementary file 1 [file BSE-PES-SI.pdf]

# Supporting Information for
# "Pros and Cons of the Bethe-Salpeter Formalism for Ground-State Energies"

Pierre-François Loos,[1,*] Anthony Scemama,[1,†] Ivan Duchemin,[2,‡] Denis Jacquemin,[3,§] and Xavier Blase[4,¶]

[1]*Laboratoire de Chimie et Physique Quantiques (UMR 5626), Université de Toulouse, CNRS, UPS, France*
[2]*Université Grenoble Alpes, CEA, IRIG-MEM-L Sim, 38054 Grenoble, France*
[3]*Laboratoire CEISAM - UMR CNRS 6230, Université de Nantes, 2 Rue de la Houssinière, BP 92208, 44322 Nantes Cedex 3, France*
[4]*Université Grenoble Alpes, CNRS, Institut NEEL, F-38042 Grenoble, France*

TABLE I. Equilibrium bond length (in bohr) of the ground state of diatomic molecules obtained at various levels of theory and basis sets. The reference CC3 and corresponding BSE@$G_0W_0$@HF data are highlighted in bold black and bold red for visual convenience, respectively. When irregularities appear in the PES, the values are reported in parenthesis and they have been obtained by fitting a Morse potential to the PES.

| | | Molecules | | | | | | | |
|---|---|---|---|---|---|---|---|---|---|
| Method | Basis | $H_2$ | LiH | LiF | HCl | $N_2$ | CO | BF | $F_2$ |
| CC3 | cc-pVDZ | 1.438 | 3.043 | 3.012 | 2.435 | 2.114 | 2.166 | 2.444 | 2.740 |
| | cc-pVTZ | 1.403 | 3.011 | 2.961 | 2.413 | 2.079 | 2.143 | 2.392 | 2.669 |
| | cc-pVQZ | **1.402** | **3.019** | **2.963** | **2.403** | **2.075** | **2.136** | **2.390** | **2.663** |
| CCSD | cc-pVDZ | 1.438 | 3.044 | 3.006 | 2.433 | 2.101 | 2.149 | 2.435 | 2.695 |
| | cc-pVTZ | 1.403 | 3.012 | 2.954 | 2.409 | 2.064 | 2.126 | 2.382 | 2.629 |
| | cc-pVQZ | 1.402 | 3.020 | 2.953 | 2.398 | 2.059 | 2.118 | 2.118 | 2.621 |
| CC2 | cc-pVDZ | 1.426 | 3.046 | 3.026 | 2.427 | 2.146 | 2.187 | 2.444 | 2.710 |
| | cc-pVTZ | 1.393 | 3.008 | 2.995 | 2.406 | 2.109 | 2.163 | 2.394 | 2.664 |
| | cc-pVQZ | 1.391 | 2.989 | 2.982 | 2.396 | 2.106 | 2.156 | 2.393 | 2.665 |
| MP2 | cc-pVDZ | 1.426 | 3.041 | 3.010 | 2.426 | 2.133 | 2.166 | 2.431 | 2.681 |
| | cc-pVTZ | 1.393 | 3.004 | 2.968 | 2.405 | 2.095 | 2.144 | 2.383 | 2.636 |
| | cc-pVQZ | 1.391 | 3.008 | 2.970 | 2.395 | 2.091 | 2.137 | 2.382 | 2.634 |
| BSE@$G_0W_0$@HF | cc-pVDZ | 1.437 | 3.042 | 3.000 | 2.454 | 2.107 | 2.153 | 2.407 | (2.698) |
| | cc-pVTZ | 1.404 | 3.023 | (2.982) | 2.410 | 2.068 | 2.116 | (2.389) | (2.647) |
| | cc-pVQZ | **1.399** | **3.017** | **(2.973)** | **2.400** | **2.065** | **2.134** | **2.383** | **(2.638)** |
| RPA@$G_0W_0$@HF | cc-pVDZ | 1.426 | 3.019 | 2.994 | 2.436 | 2.083 | 2.144 | 2.403 | (2.629) |
| | cc-pVTZ | 1.388 | 2.988 | (2.965) | 2.408 | 2.055 | 2.114 | (2.370) | (2.584) |
| | cc-pVQZ | 1.382 | 2.997 | (2.965) | 2.370 | 2.043 | 2.132 | 2.367 | (2.571) |
| RPAx@HF | cc-pVDZ | 1.428 | 3.040 | 2.998 | 2.424 | 2.077 | 2.130 | 2.417 | 2.611 |
| | cc-pVTZ | 1.395 | 3.003 | 2.943 | 2.400 | 2.046 | 2.110 | 2.368 | 2.568 |
| | cc-pVQZ | 1.394 | 3.011 | 2.944 | 2.391 | 2.041 | 2.104 | 2.366 | 2.565 |
| RPA@HF | cc-pVDZ | 1.431 | 3.021 | 2.999 | 2.424 | 2.083 | 2.134 | 2.416 | 2.623 |
| | cc-pVTZ | 1.388 | 2.978 | 2.939 | 2.396 | 2.045 | 2.110 | 2.362 | 2.579 |
| | cc-pVQZ | 1.386 | 2.994 | 2.946 | 2.382 | 2.042 | 2.103 | 2.364 | 2.573 |

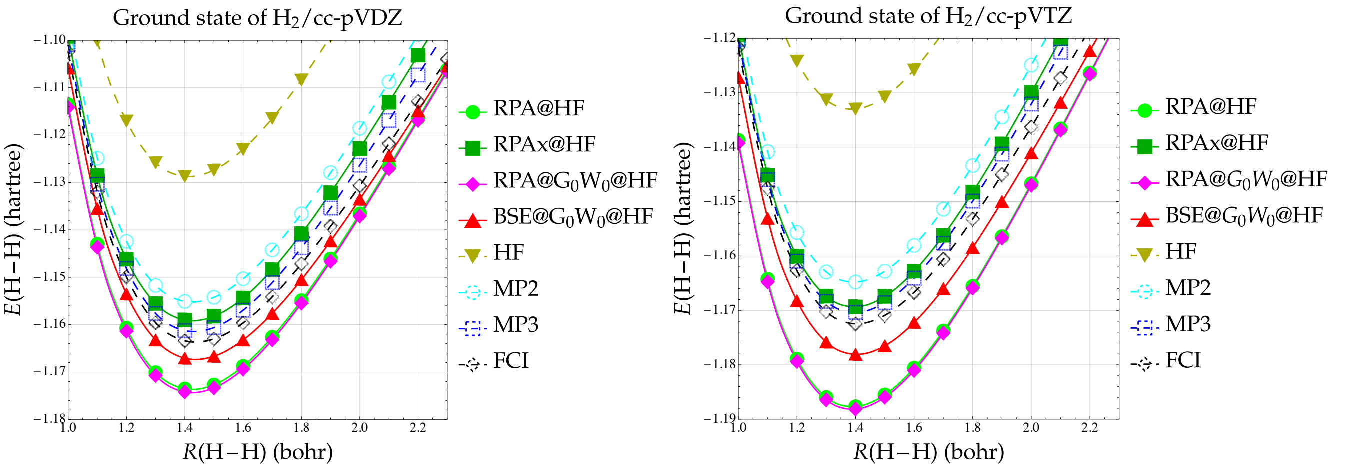


FIG. 1. Ground-state potential energy surfaces of $H_2$ around its respective equilibrium geometry obtained at various levels of theory and basis sets.


* loos@irsamc.ups-tlse.fr
† scemama@irsamc.ups-tlse.fr
‡ ivan.duchemin@cea.fr
§ denis.jacquemin@univ-nantes.fr
¶ xavier.blase@neel.cnrs.fr


[1] Holzer, C.; Gui, X.; Harding, M. E.; Kresse, G.; Helgaker, T.; Klopper, W. Bethe–Salpeter Correlation Energies of Atoms and Molecules. *J. Chem. Phys.* **2018**, *149*, 144106.

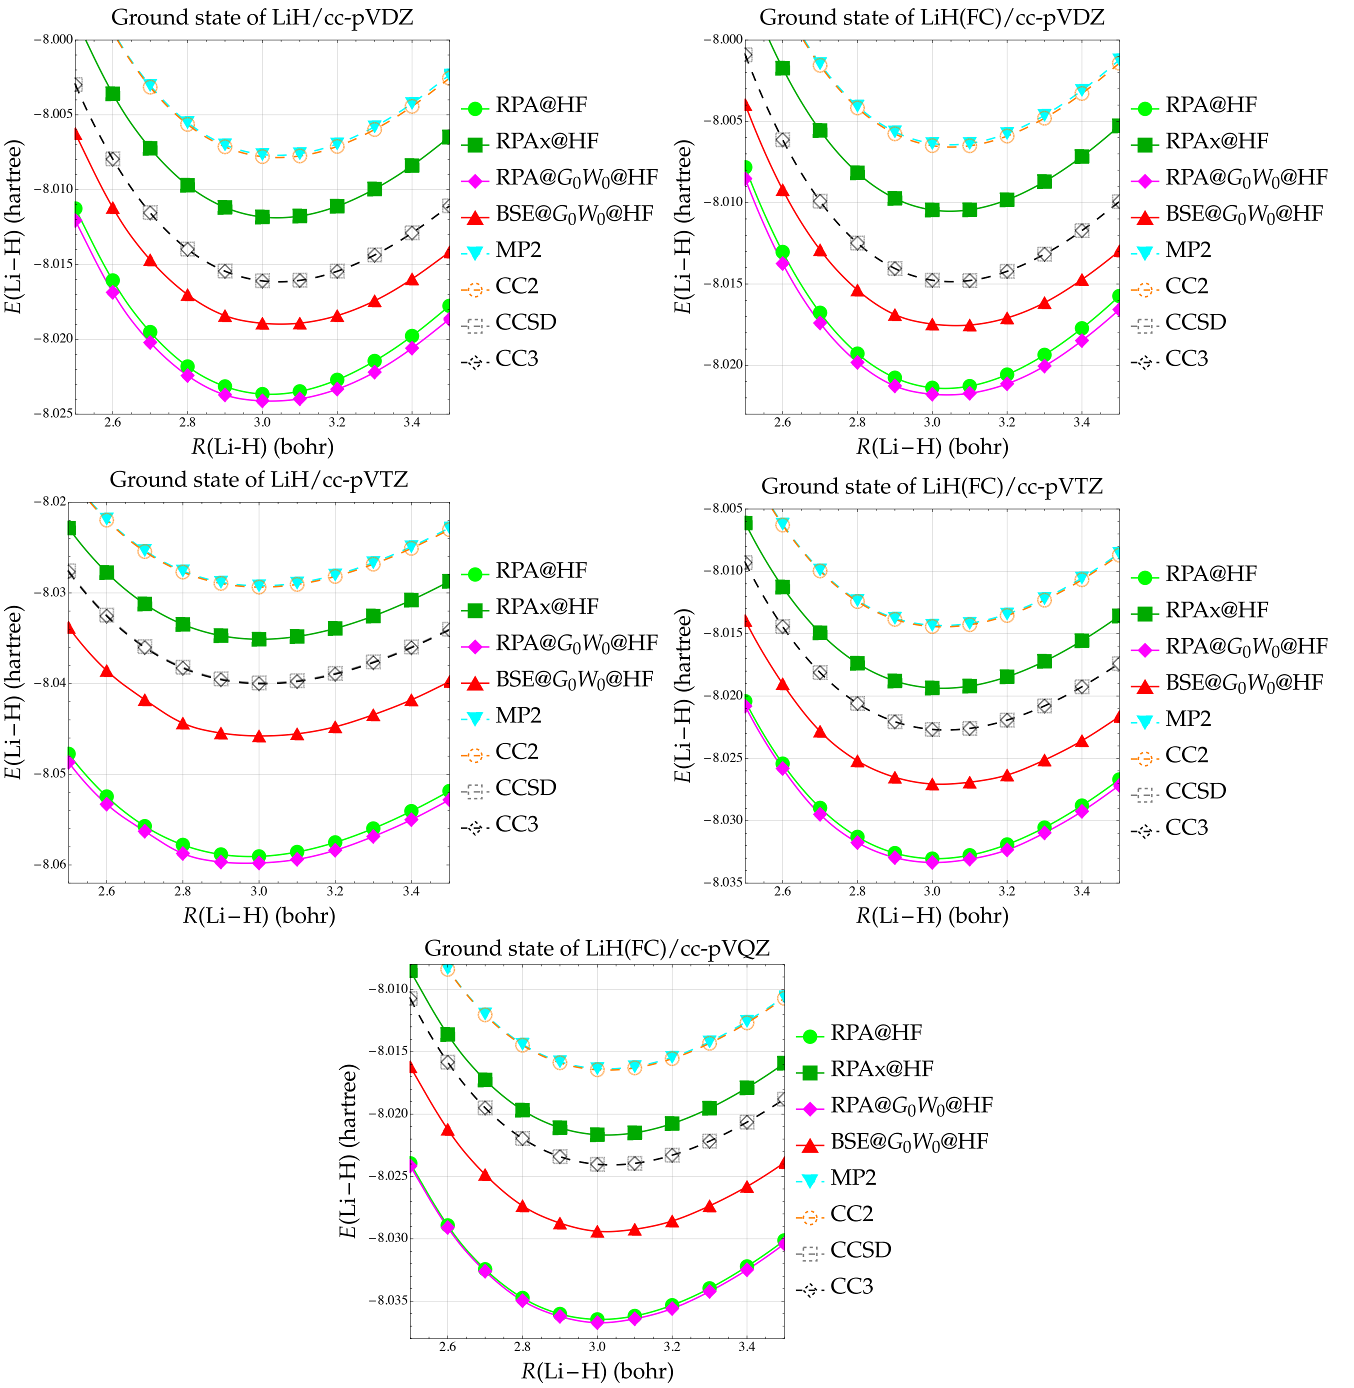


FIG. 2. Ground-state potential energy surfaces of LiH around its respective equilibrium geometry obtained at various levels of theory and basis sets. FC stands for frozen core.

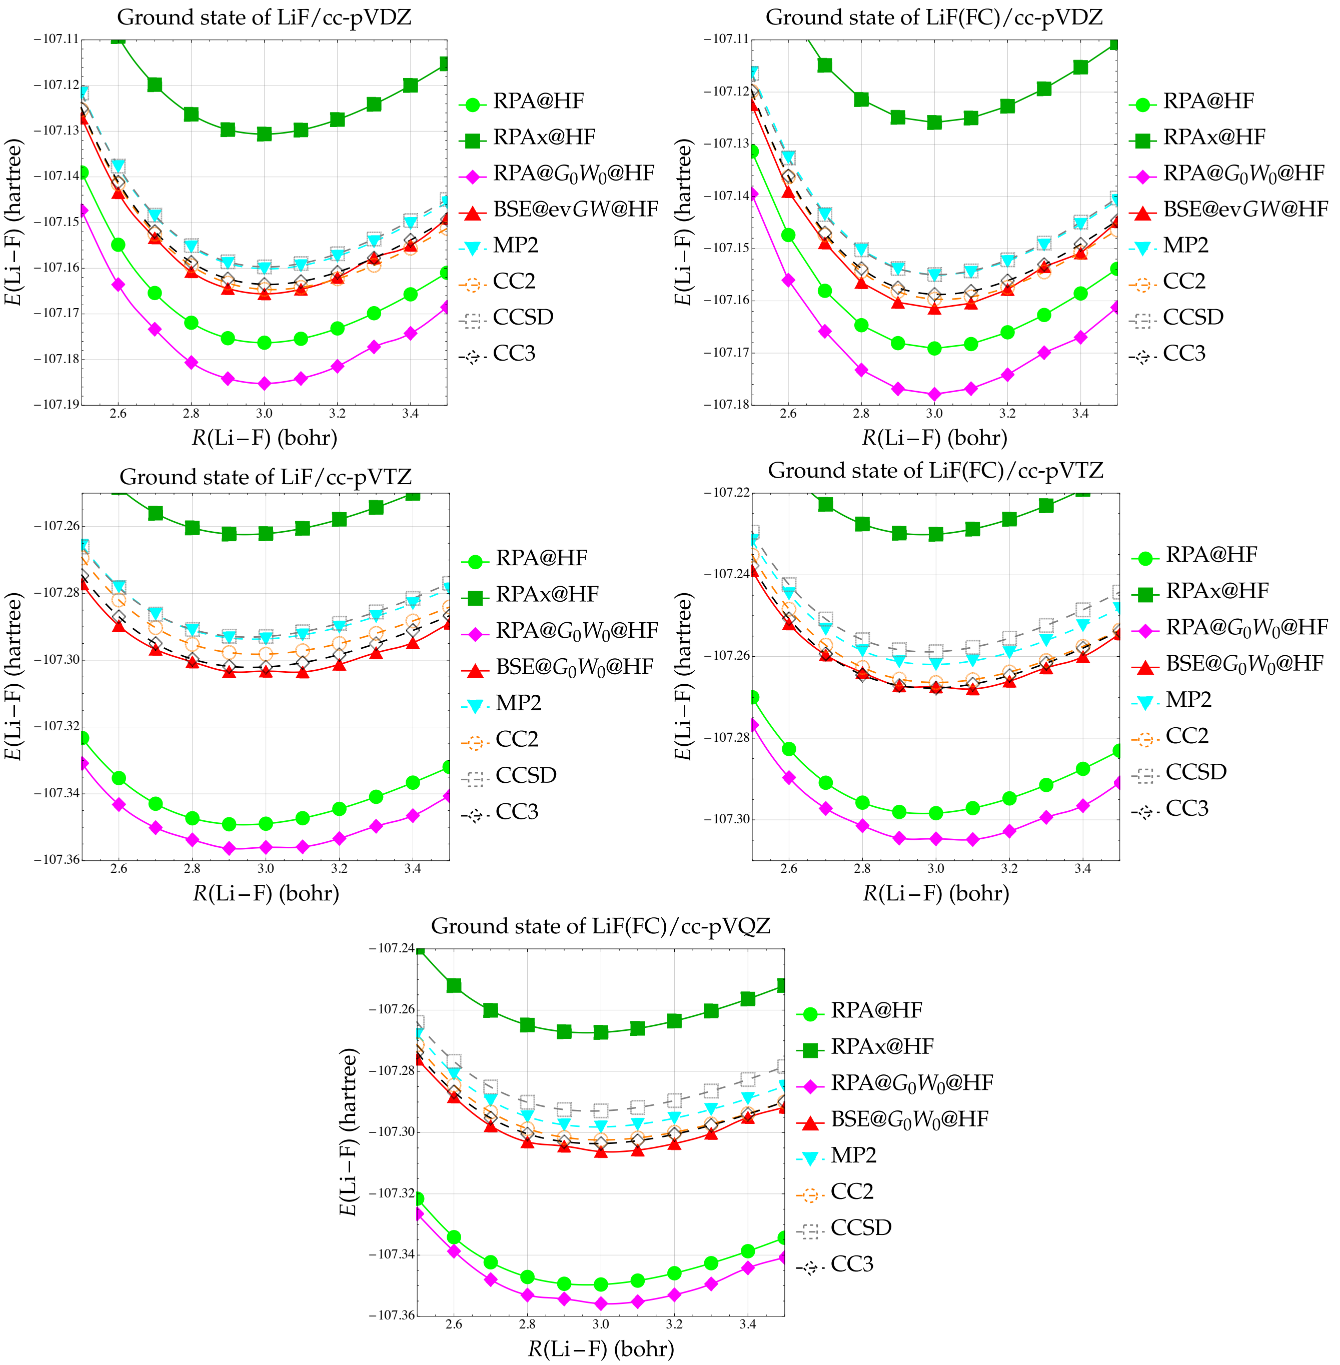


FIG. 3. Ground-state potential energy surfaces of LiF around its respective equilibrium geometry obtained at various levels of theory and basis sets. FC stands for frozen core.

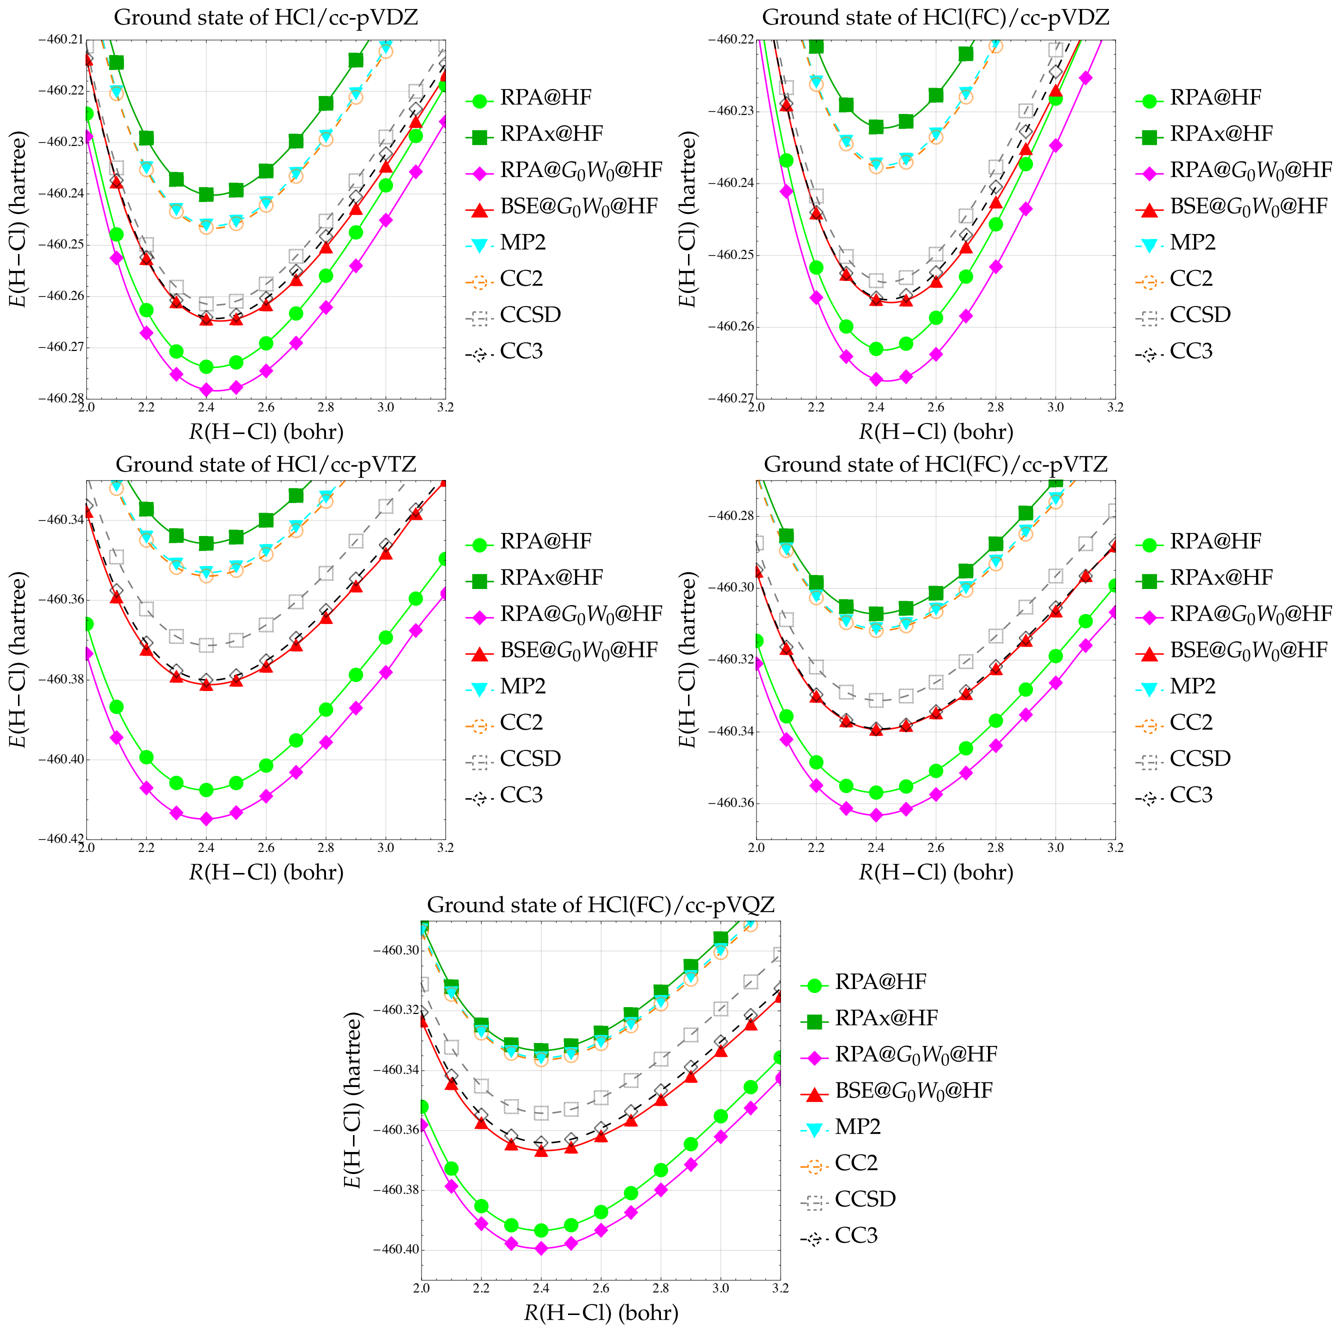


FIG. 4. Ground-state potential energy surfaces of HCl around its respective equilibrium geometry obtained at various levels of theory and basis sets. FC stands for frozen core.

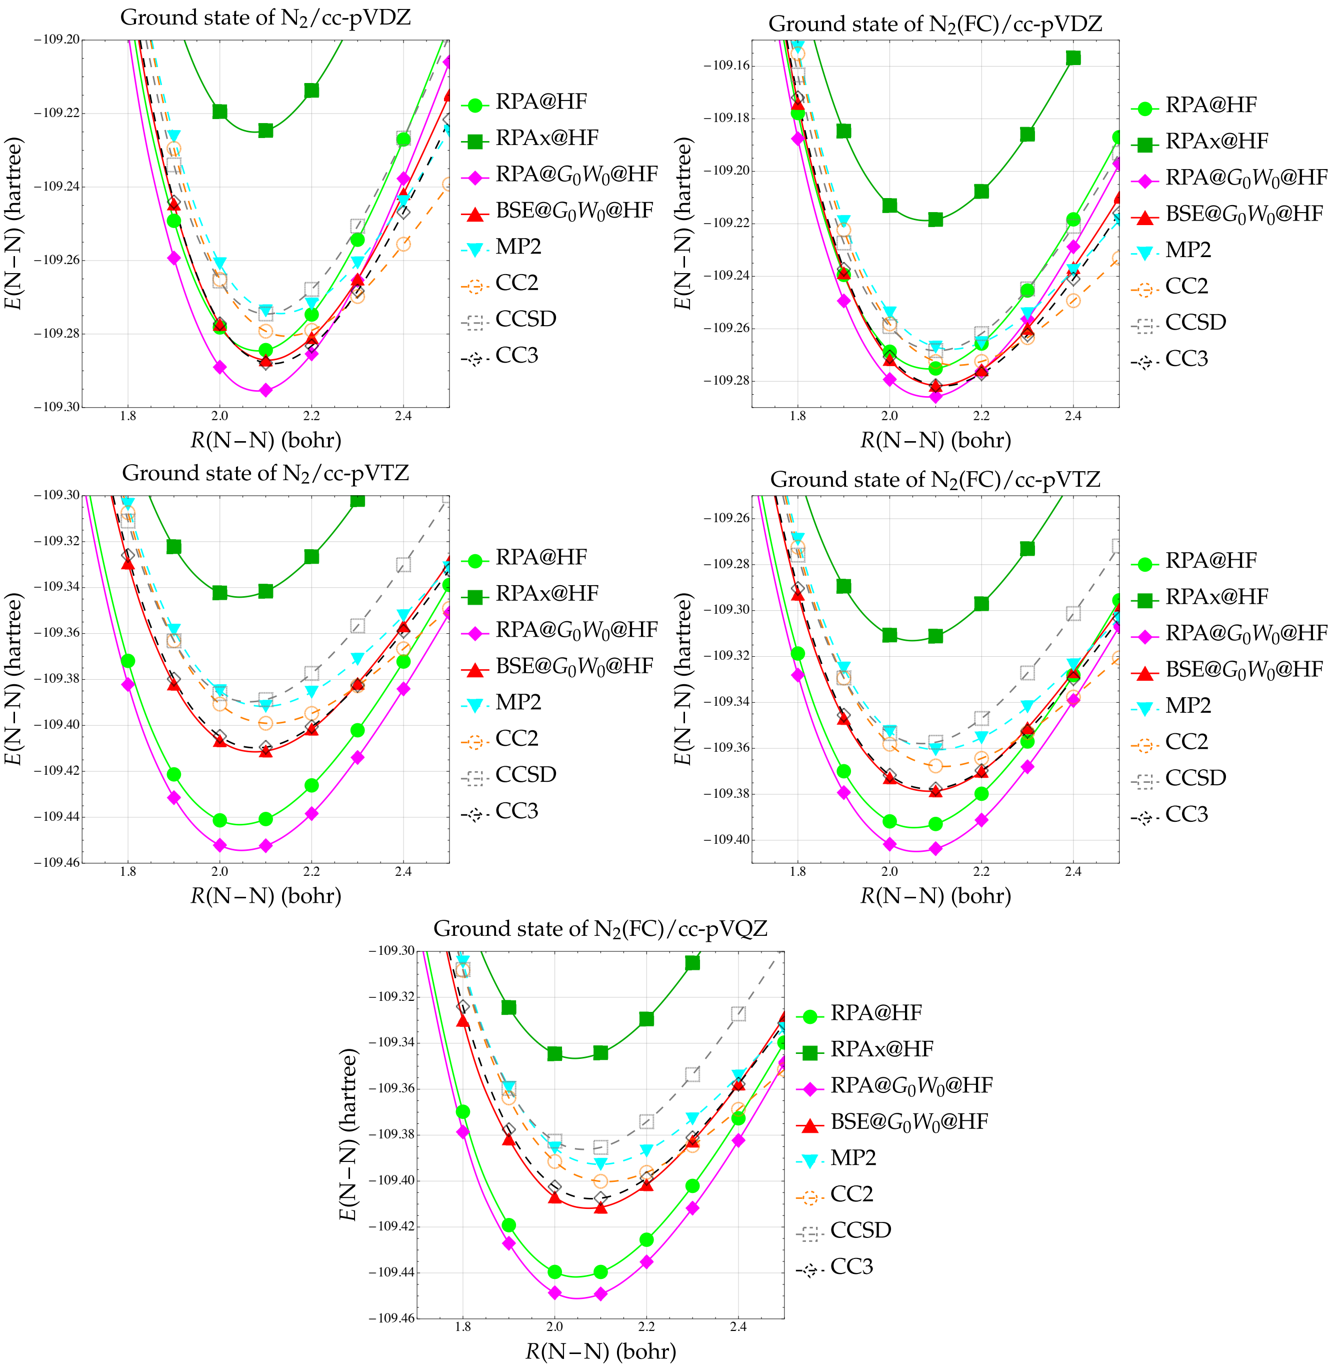


FIG. 5. Ground-state potential energy surfaces of $N_2$ around its respective equilibrium geometry obtained at various levels of theory and basis sets. FC stands for frozen core.

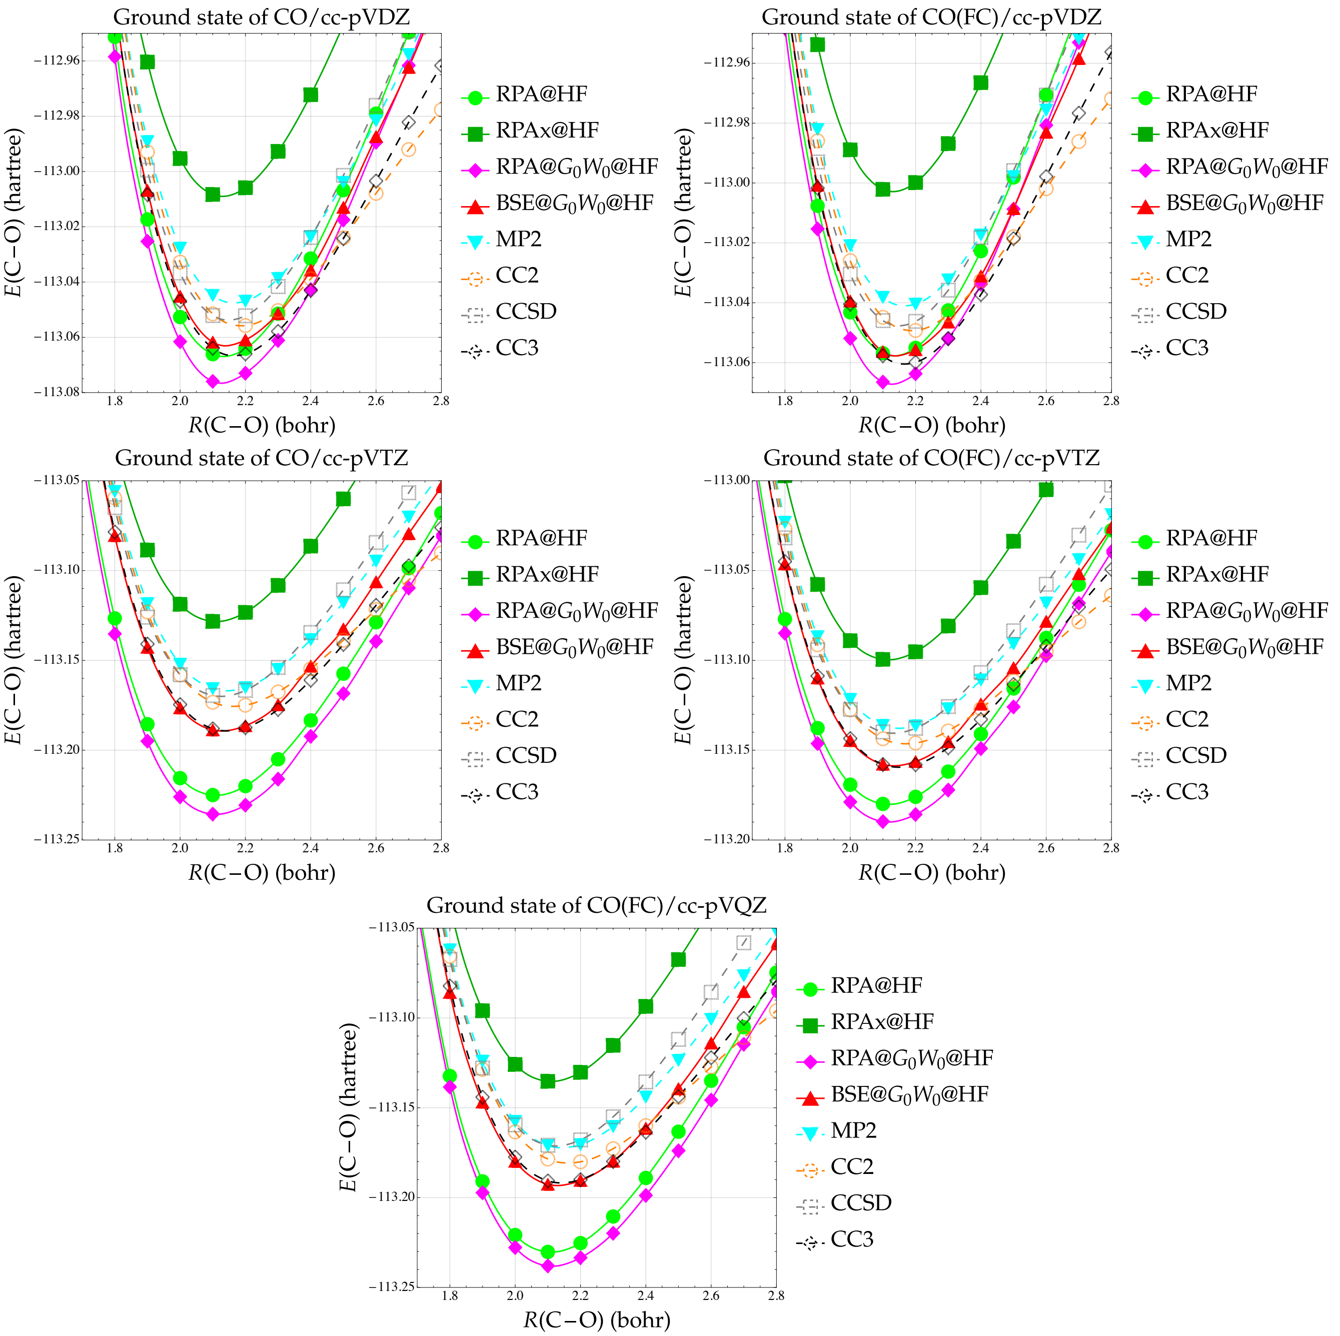


FIG. 6. Ground-state potential energy surfaces of CO around its respective equilibrium geometry obtained at various levels of theory and basis sets. FC stands for frozen core.

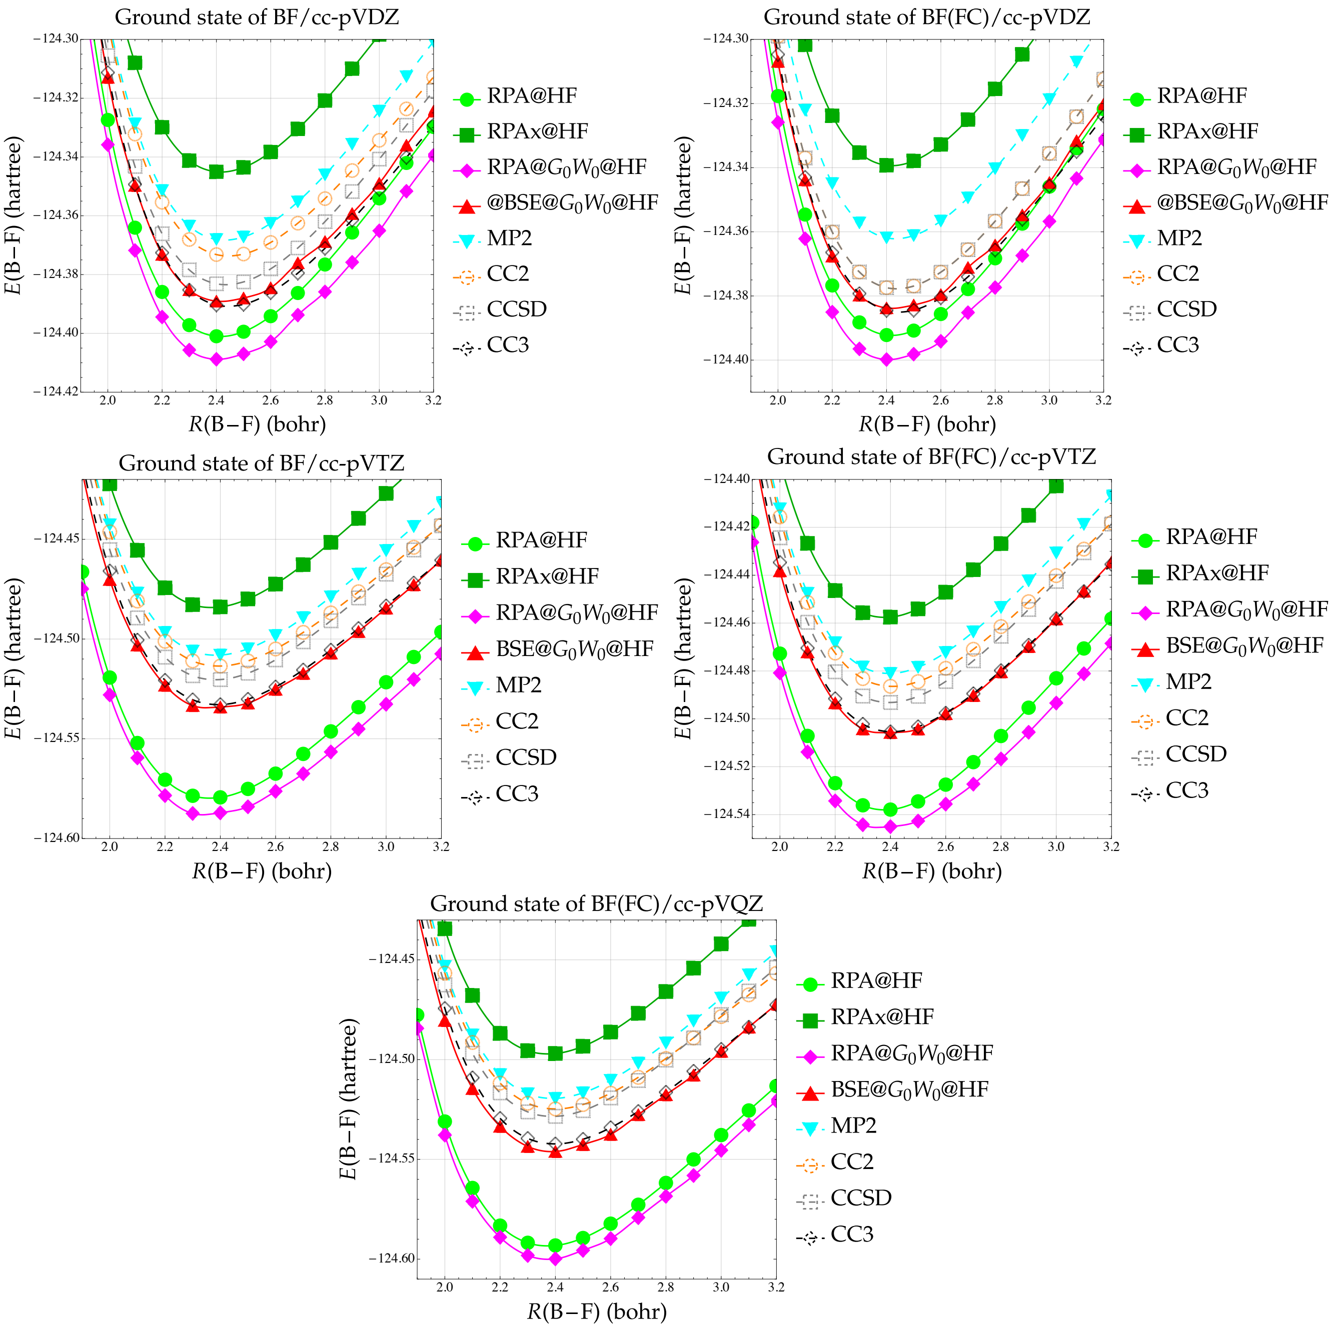


FIG. 7. Ground-state potential energy surfaces of BF around its respective equilibrium geometry obtained at various levels of theory and basis sets. FC stands for frozen core.

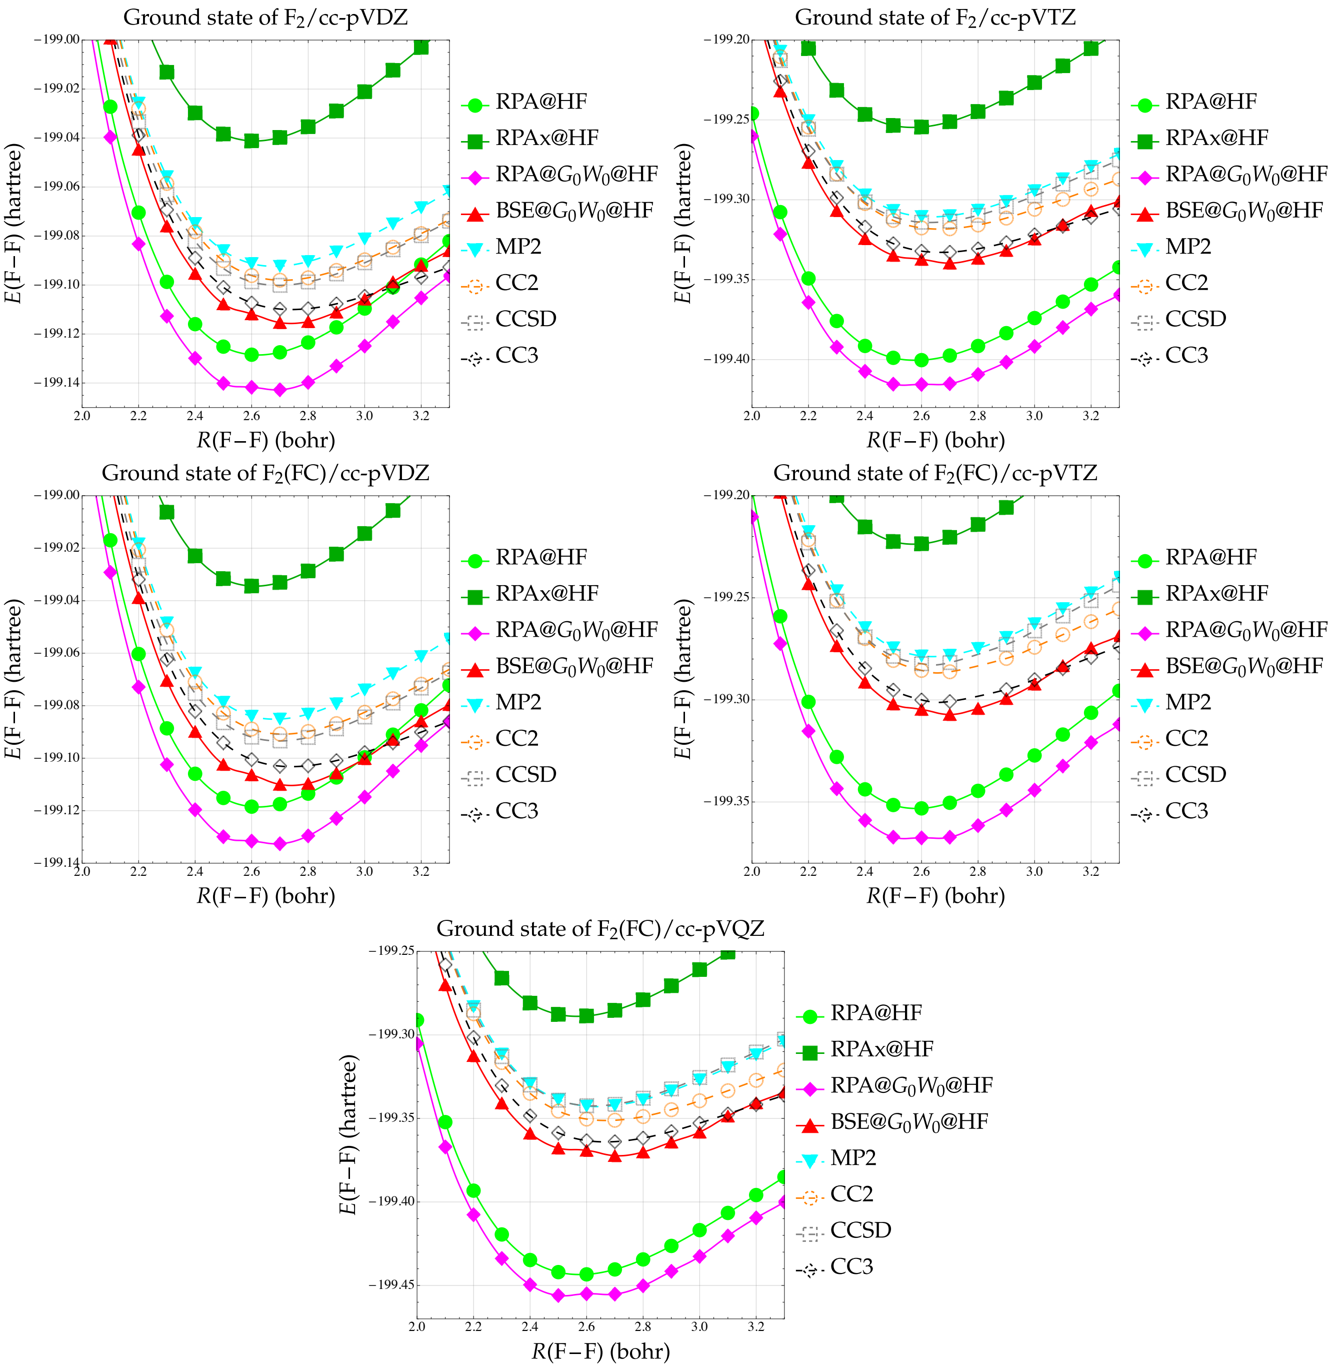


FIG. 8. Ground-state potential energy surfaces of $F_2$ around its respective equilibrium geometry obtained at various levels of theory and basis sets. FC stands for frozen core.

TABLE II. Ground-state total and correlation energies obtained at various levels of theory for diatomic molecules at their equilibrium geometry. All the calculations have been performed without frozen-core approximation with the cc-pVQZ basis set.

| System | Geometry | Method | Energy (Ha) | $-E_c$ (mHa) | Error wrt CC3 (%) |
|---|---|---|---|---|---|
| $H_2$ | $R_{H-H} = 1.402$ | HF | −1.133 458 | | |
| | | CC3 | −1.173 840 | 40.4 | |
| | | CCSDT | −1.173 840 | 40.4 | 0.0% |
| LiH | $R_{Li-H} = 3.019$ | HF | −7.987 235 | | |
| | | CC3 | −8.057 209 | 70.0 | |
| | | CCSDT | −8.057 233 | 70.0 | 0.0% |
| | | CCSDT(Q) | −8.057 233 | 70.0 | 0.0% |
| | | CCSDTQ | −8.057 233 | 70.0 | 0.0% |
| LiF | $R_{Li-F} = 2.963$ | HF | −106.990 854 | | |
| | | CC3 | −107.374 540 | 383.7 | |
| | | CCSDT | −107.373 314 | 382.5 | −0.3% |
| | | CCSDT(Q) | −107.373 701 | 382.9 | −0.2% |
| HCl | $R_{H-Cl} = 2.403$ | HF | −460.111 442 | | |
| | | CC3 | −460.493 630 | 382.2 | |
| | | CCSDT | −460.493 675 | 382.2 | +0.0% |
| | | CCSDT(Q) | −460.494 110 | 382.7 | +0.1% |
| $N_2$ | $R_{N-N} = 2.075$ | HF | −108.991 326 | | |
| | | CC3 | −109.485 718 | 494.4 | |
| | | CCSDT | −109.484 058 | 492.7 | −0.3% |
| | | CCSDT(Q) | −109.486 040 | 494.7 | +0.1% |
| CO | $R_{C-O} = 2.136$ | HF | −112.788 718 | | |
| | | CC3 | −113.266 297 | 477.6 | |
| | | CCSDT | −113.264 330 | 475.6 | −0.4% |
| | | CCSDT(Q) | −113.265 613 | 476.9 | −0.1% |
| BF | $R_{B-F} = 2.390$ | HF | −124.166 127 | | |
| | | CC3 | −124.613 599 | 447.5 | |
| | | CCSDT | −124.612 523 | 446.4 | −0.2% |
| | | CCSDT(Q) | −124.613 118 | 447.0 | −0.1% |
| $F_2$ | $R_{F-F} = 2.663$ | HF | −198.769 005 | | |
| | | CC3 | −199.437 880 | 668.9 | |
| | | CCSDT | −199.437 033 | 668.0 | +0.1% |
| | | CCSDT(Q) | −199.438 815 | 669.8 | −0.1% |

TABLE III. Comparison between the extended (XBS) and regular BSE schemes, as defined in Ref. 1. The calculations have been performed at the XBS equilibrium geometries. Note that the methodology presented in the present paper is theoretically equivalent to the XBS scheme. All the calculations have been performed without frozen-core approximation with the cc-pVQZ basis set.

| System | Geometry | Method | $-E_c$ (mHa) | Error wrt CC3 (%) |
|---|---|---|---|---|
| $H_2$ | $R_{H-H} = 1.399$ | BSE | 46.5 | +15.1% |
| | | XBS | 47.2 | +16.9% |
| LiH | $R_{Li-H} = 3.017$ | BSE | 78.0 | +11.4% |
| | | XBS | 78.1 | +11.6% |
| LiF | $R_{Li-F} = 2.973$ | BSE | 388.3 | +1.2% |
| | | XBS | 385.0 | +0.4% |
| HCl | $R_{H-Cl} = 2.400$ | BSE | 385.1 | +0.8% |
| | | XBS | 384.5 | +0.6% |
| $N_2$ | $R_{N-N} = 2.065$ | BSE | 493.7 | −0.1% |
| | | XBS | 497.9 | +0.7% |
| CO | $R_{C-O} = 2.134$ | BSE | 476.2 | −0.3% |
| | | XBS | 480.0 | +0.5% |
| BF | $R_{B-F} = 2.385$ | BSE | 450.0 | +0.6% |
| | | XBS | 452.3 | +1.1% |
| $F_2$ | $R_{F-F} = 2.638$ | BSE | 670.3 | 0.2% |
| | | XBS | 673.9 | 0.8% |
